# Supplementary material for: A recurrent vision transformer shows signatures of primate visual attention
Source: arXiv:2502.10955 source file (2025-02-16)
Supplement: Supplementary file 4 [file SuppValue.tex]

\documentclass[12pt]{article}

\usepackage{amsmath,amsfonts,amssymb,mathtools}
\usepackage{algorithm,algpseudocode}
\usepackage{hyperref,xcolor,graphicx,gensymb}
\usepackage{microtype,geometry}
\geometry{a4paper, margin=1in}

\begin{document}

\title{Supplementary Information: Distributional Value and Self-Attention}
\date{\today}
\maketitle

\section{Distributional Reinforcement Learning in Offline Settings}

\subsection{Distributional Value Functions}

In traditional reinforcement learning, we typically estimate the expected value function $V^\pi(s) = \mathbb{E}[G_t | S_t = s]$, where $G_t$ is the discounted cumulative reward from time step $t$ onwards. However, this expectation fails to capture the full complexity of possible outcomes. Distributional reinforcement learning (DRL) addresses this limitation by learning the entire distribution of returns, denoted as $Z^\pi(s)$.

Mathematically, we represent this distribution as:

\begin{equation}
Z^\pi(s) \stackrel{D}{=} R(s, A) + \gamma Z^\pi(S')
\end{equation}

where $A \sim \pi(\cdot|s)$ is the action selected according to policy $\pi$, $S' \sim P(\cdot|s,A)$ is the next state following the environment dynamics $P$, and $\stackrel{D}{=}$ denotes equality in distribution. This equation encapsulates the idea that the return distribution for a state is composed of the immediate reward plus the discounted return distribution of the next state.

The distributional Bellman operator $\mathcal{T}^\pi$ formalizes this relationship:

\begin{equation}
\mathcal{T}^\pi Z(s) \stackrel{D}{=} R(s, A) + \gamma Z(S')
\end{equation}

This operator maps one return distribution to another, incorporating the immediate reward and the discounted future returns.

\subsection{Categorical Distribution and Projection}

To make the distributional approach computationally tractable, we approximate $Z^\pi$ using a categorical distribution over a fixed set of atoms $\{z_1, ..., z_K\}$. These atoms represent possible return values, and their associated probabilities form our approximation of the return distribution.

The projection operator $\Phi_z : \mathcal{P}(\mathbb{R}) \to \mathcal{P}(z)$ is crucial in this approximation. It maps any distribution onto our fixed set of atoms. For a distribution $\eta$, the projection is defined as:

\begin{equation}
(\Phi_z \eta)_i = \sum_{j=0}^{K-1} [\frac{u_j - z_i}{\Delta z}]_0^1 p_j
\end{equation}

Here, $[x]_0^1 = \max(0, \min(1, x))$ is a clipping function, $\Delta z$ is the distance between atoms, and $u_j = r + \gamma z_j$ represents the combination of immediate reward and discounted future return.

This projection distributes probability mass from the true distribution to the nearest atoms in our approximation, preserving the overall shape of the distribution while constraining it to our chosen support.

\subsection{Distributional Q-Learning in Offline Settings}

In the offline setting, we adapt the distributional Q-learning update to use a fixed dataset $\mathcal{D}$ of previously collected experiences. The update for the parameterized distribution $Z_\theta$ becomes:

\begin{equation}
\theta \leftarrow \theta + \alpha \nabla_\theta D_{KL}(\Phi_z \mathcal{T}^\pi Z_{\theta'}(s, a) \| Z_\theta(s, a))
\end{equation}

where $(s, a, r, s') \sim \mathcal{D}$ is a transition sampled from the offline dataset, $\theta'$ are the parameters of a target network (used for stability in learning), and $D_{KL}$ is the Kullback-Leibler divergence.

This update aims to minimize the difference between our current estimate $Z_\theta(s, a)$ and the target distribution $\Phi_z \mathcal{T}^\pi Z_{\theta'}(s, a)$, which is the projected Bellman update of our target network's estimate.

\subsection{Loss Function Formulation}

Our loss function integrates the distributional Q-learning update with policy improvement and entropy regularization:

\begin{equation}
\mathcal{L}(\theta) = \mathcal{L}_{KL} + \lambda_1 \mathcal{L}_{pol} + \lambda_2 \mathcal{L}_{H}
\end{equation}

The KL-divergence term $\mathcal{L}_{KL}$ is defined as:

\begin{equation}
\mathcal{L}_{KL} = \mathbb{E}_{(s,a,r,s') \sim \mathcal{D}}[D_{KL}(\Phi_z \mathcal{T}^\pi Z_{\theta'}(s, a) \| Z_\theta(s, a))]
\end{equation}

This term encourages our current estimate to match the projected Bellman update, averaged over transitions in our dataset.

The policy improvement term $\mathcal{L}_{pol}$ is:

\begin{equation}
\mathcal{L}_{pol} = -\mathbb{E}_{s \sim \mathcal{D}, a \sim \pi_\theta(\cdot|s)}[\mathbb{E}[Z_\theta(s,a)]]
\end{equation}

This term encourages the policy to select actions that maximize the expected return according to our current value estimates.

The entropy regularization term $\mathcal{L}_{H}$ is:

\begin{equation}
\mathcal{L}_{H} = -\mathbb{E}_{s \sim \mathcal{D}}[H(\pi_\theta(\cdot|s))]
\end{equation}

where $H(\cdot)$ is the entropy function. This term promotes exploration and prevents premature convergence to deterministic policies, which is particularly important in offline settings where we cannot actively explore the environment.

\subsection{Target Distribution Computation}

The target distribution, which serves as our learning target, is computed as:

\begin{equation}
(\Phi_z \mathcal{T}^\pi Z_{\theta'}(s, a))_i = \sum_{j=0}^{K-1} [\frac{r + \gamma z_j - z_i}{\Delta z}]_0^1 p_j(s', a')
\end{equation}

where $a' \sim \pi_\theta(\cdot|s')$ is an action sampled from our current policy in the next state, and $p_j(s', a')$ is the probability mass on atom $z_j$ for state-action pair $(s', a')$ according to the target network $Z_{\theta'}$.

This equation represents the projection of the Bellman update onto our fixed set of atoms. It combines the observed reward $r$ with the discounted future return estimates $\gamma z_j$, distributing probability mass to the nearest atoms in our support.

\section{Value and Self-Attention}

The integration of self-attention mechanisms with distributional reinforcement learning offers a powerful framework for capturing complex dependencies in the state space while also modeling the uncertainty in value estimates. Figure \ref{fig:LogitsS1Attention} illustrates the effect of attentional modulation on the actor network's logits for changes in stimulus $S_1$.

In our architecture, the self-attention mechanism operates on a set of input tokens $x_1, ..., x_n$, each representing different aspects of the state. The attention weights are computed as:

\begin{equation}
\alpha_{ij} = \frac{\exp(e_{ij})}{\sum_k \exp(e_{ik})}
\end{equation}

where $e_{ij} = \frac{(W_Q x_i)^T (W_K x_j)}{\sqrt{d_k}}$, with $W_Q$ and $W_K$ being learnable weight matrices and $d_k$ the dimension of the key vectors.

These attention weights modulate the information flow in the network, allowing it to focus on relevant parts of the state for different decisions. The output of the self-attention layer for token $i$ is given by:

\begin{equation}
y_i = \sum_j \alpha_{ij} (W_V x_j)
\end{equation}

where $W_V$ is another learnable weight matrix.

The self-attention mechanism interacts with our distributional value estimates by influencing the learned representations that are used to predict the return distribution. Specifically, the output of the self-attention layers feeds into the networks that parameterize our categorical distribution over returns.

Let $\phi(s)$ be the state representation after applying self-attention. Our value distribution estimate becomes:

\begin{equation}
Z_\theta(s,a) = \text{Categorical}(z_1, ..., z_K; p_\theta(\phi(s), a))
\end{equation}

where $p_\theta$ is a neural network that outputs the probabilities for each atom, conditioned on the attended state representation and the action.

This formulation allows the network to attend to different aspects of the state when estimating the return distribution for different actions. As shown in Figure \ref{fig:LogitsS1Attention}, changes in the attended stimulus $S_1$ lead to corresponding changes in the actor's logits, demonstrating how attention mechanisms can capture the relevance of different state components for decision-making.

The combination of distributional RL and attention mechanisms provides a flexible framework for learning complex value functions and policies from offline data. It allows the agent to capture both the uncertainty in returns and the relevant features of high-dimensional state spaces, potentially leading to more robust and efficient learning in complex environments.

\section{Self-Attention, Value, and Uncertainty}
\begin{figure}[htbp]
    \centering
    \includegraphics[width=0.99\linewidth]{suppFigures/attention_value_entropy_one.png}
    \caption{      
    }
    \label{fig:ValuevsAttention}
\end{figure}

\end{document}
